# Supplementary material for: LAC: Latent Action Composition for Skeleton-based Action Segmentation
Source: arXiv:2308.14500 source file (2024-02-21)
Supplement: Supplementary file 1 [file Appendix.tex]

\noindent\textbf{Posetics}~\cite{unik} is created on top of Kinetics-400~\cite{Carreira_2017_CVPR} videos. It contains 142,000 real-world video clips of 320 action classes with the corresponding 2D and 3D skeletons. We use the Posetics dataset to pre-train LAC framework with skeleton data and we study the transfer-learning on skeleton-based action segmentation on downstream tasks. 
\vspace{0.1cm}

\noindent\textbf{Toyota Smarthome Untrimmed (TSU)}~\cite{Dai_2022_PAMI} is a real-world dataset for daily living action segmentation recorded in indoor environment. The dataset contains 536 videos with 51 densely annotated long-term composite activities where up to 5 actions can happen at the same time in a given frame. We only use the officially provided 2D skeleton data~\cite{Yang_2021_WACV} for the experiments. For the evaluation, we report \textit{per-frame}
mAP (mean Average Precision) as~\cite{dai2021pdan, dai2022mstct} following the cross-subject (CS) and cross-view (CV) evaluation protocols.
\vspace{0.1cm}

\noindent\textbf{Charades}~\cite{Sigurdsson2016HollywoodIH} is a large dataset with 9848 videos of daily indoor actions. The dataset contains 66,000+ temporal annotations for 157 action classes, with a high overlap among action instances of different classes. This dataset provides only raw video clips without skeleton data. In this work we are focusing on skeleton based action segmentation, so we use the estimated 2D skeleton data (2D coordinates) using the toolbox~\cite{Yang_2021_WACV} as our input and discard the raw RGB frames. For the multi-person
cases, we select 2 people with the highest average joint confidence in each clip follwing~\cite{Yan2018SpatialTG}. We report \textit{per-frame} mAP on the localization setting of the dataset. We will release the estimated skeleton data on Charades for reproducing the results.

\vspace{0.1cm}

\noindent\textbf{PKU-MMD}~\cite{liu2017pku} is the basic skeleton-based action detection dataset recorded in the laboratory setting. It contains 1,076 long untrimmed video sequences performed by 66 subjects in three camera views. 51 action categories are annotated. We use only the official 3D skeleton data for our framework. As this dataset is not densely labeled, we report the event-based mAP for fair comparisons by performing a post-processing step on top of the frame-level predictions to generate the action boundaries.

\vspace{0.1cm}
\noindent\textbf{Mixamo}~\cite{mixamo} is a 3D animation collection, which contains approximately 2,400 unique motion sequences, including elementary actions, and various dancing moves. Each of these motions may be applied to 71 distinct characters, which share a human skeleton topology, but may differ in their body size and proportions. We use such a synthetic dataset, which includes the motion retargeting ground truth for pre-training and evaluating the generation module in LAC.
